# Supplementary material for: Individual preventive measures during an epidemic may have negative population-level outcomes
Source: arXiv:1805.05211 ancillary file (2018-05-14)
Supplement: Supplementary file 1 [file socialdistancing_suppl.pdf]

# Supplementary Information

# Individual preventive measures during an epidemic may have negative population-level outcome

Ka Yin Leung[a,1], Frank Ball[2], David Sirl[2], and Tom Britton[1]

30th April 2018

## Section S1 Configuration network

### Section S1.1 Notation and construction

The (Newman-Strogatz-Watts version of the) configuration model is defined in the main text in Section 2.2.1. The degree $D$ of an individual in the network is distributed as the pre-defined distribution $\{p_d\}$. The mean and variance of $D$ are denoted by $\mu_D$ and $\sigma_D^2$, respectively. In the configuration network construction a given half-edge is $d$ times as likely to be paired with a given individual with degree $d$ than with a given individual with degree 1. Therefore, a neighbour has size-biased degree $\tilde{D}$, where $P(\tilde{D} = d) = dp_d/\mu_D$, $d = 1, 2, \ldots$ The configuration model is well studied, e.g. [7]. It is for instance known that, as the population size $n \to \infty$, there will be zero connected components that have size of exact order $n$ if $\mu_D + \sigma_D^2/\mu_D - 1 \leq 1$, and precisely one connected component of exact order $n$ if $\mu_D + \sigma_D^2/\mu_D - 1 > 1$. Since there is at most one component that has size of exact order $n$ this component is often called the giant component. Further, if the degrees are not small, then the giant often makes up close to all individuals. If for example all individuals have the same degree $d > 2$, then exactly every node is part of the giant component with a probability tending to 1.

### Section S1.2 Epidemic threshold parameter $R_0$

The basic reproduction number $R_0$ for the configuration network model with rewiring and dropping has been derived previously in [8]:

$$R_0 = \frac{\beta}{\beta + \omega + \gamma}\left(\mu_D + \frac{\sigma_D^2}{\mu_D} - 1\right). \tag{S.1}$$

This formula is easily interpreted as follows. Observe that $\beta/(\beta + \omega + \gamma)$ is the probability that transmission occurs before social distancing or recovery (note that for an infected individual it

[a]kayin.leung@math.su.se
[1]Department of Mathematics, Stockholm University, 106 91 Stockholm, Sweden
[2]School of Mathematical Sciences, University of Nottingham, University Park, Nottingham NG7 2RD, UK

does not matter whether social distancing is through dropping or rewiring since he/she loses one of his/her neighbours either way). A newly infected individual has size-biased degree $\tilde{D}$. Note that the number of susceptible neighbours of a newly infected individual is $\tilde{D} - 1$. The mean of $\tilde{D} - 1$ is equal to $\mu_D + \sigma_D^2/\mu_D - 1$. Therefore, the expected number of secondary cases generated by a typical newly infected individual is given by (S.1). From (S.1) we see that $R_0$ is a monotonically decreasing function of $\omega$, i.e. any social distancing always reduces $R_0$. In particular, if $R_0$ is larger than one in the baseline setting without any social distancing ($\omega = 0$), then social distancing reduces $R_0$ to below its epidemic threshold of one if and only if $\omega \geq \beta(\mu_D + \sigma_D^2/\mu_D - 1) - \gamma$. Therefore, social distancing is always beneficial at the beginning of an epidemic in the configuration network.

## Section S1.3 Asymptotic lower bound for the final size

Assume that the degree distribution of the population only takes on values 0 and $d$, so $p_0 = 1 - p_d$ with $d > 2$. For ease of argument we consider the asymptotic lower bound only for the simplest setting of our model. We work with the special case when $\gamma = 0$ and $\omega_d = 0$, i.e. an SI infection (without recovery) and social distancing is always through rewiring to new individuals. By continuity arguments, the conclusions also hold for sufficiently small $\gamma > 0$ and $\omega_d > 0$. The degree of an individual may change over the course of an epidemic owing to rewiring. We say that an individual has 'original degree' 0 or $d$ if that was the degree of the individual in the configuration-network construction before the epidemic.

We consider $R_0$ as a function of $\omega_r$. In the setting of this section, $R_0 = R_0(\omega_r) = \beta/(\beta + \omega_r)(d-1)$ (in the early stages of the epidemic, all newly infected individuals have degree $d$). Note that $R_0(0) = d - 1$, i.e. in an SI epidemic without rewiring, a newly infected individual transmits infection to all its susceptible neighbours. Note that $R_0(0) > 1$ if and only if $d > 2$ (here we assume that $d > 2$ and hence that $R_0(0) > 1$). Let $\bar{Z}_n(\omega_r)$ denote the final fraction of the population that gets infected in the model with population size $n$ and rewiring rate $\omega_r$. If $\omega_r = 0$, then only transmission can occur (recall that we consider $\gamma = 0$), so an index case will generate an outbreak of the size equal to the size of the connected component this index case is part of. Asymptotically, as population size $n \to \infty$, as mentioned earlier, all individuals with degree $d$ will be part of the giant component of the network so the giant component consists of a fraction $p_d$ of the entire population. Therefore, as $n$ tends to infinity, $\bar{Z}_n(0)$ tends to a two-point distribution $\bar{Z}(0)$ with $P(\bar{Z}(0) = 0) = p_0 = 1 - P(\bar{Z}(0) = p_d)$. That is, in the setting without recovery, the asymptotic final fraction getting infected is either zero (if the index case has degree 0) or $p_d$ (if the index case has degree $d$).

Note that for large enough $\omega_r$, $R_0(\omega_r) < 1$. We consider $\omega_r > 0$ sufficiently small such that $R_0(\omega_r) > 1$. Furthermore, we assume that a major outbreak occurs. Therefore we assume that the index case has degree $d$ (if the index case has degree 0, then the final fraction $\bar{Z}_n(\omega)$ tends to zero as $n$ tends to infinity). Then the final fraction $\bar{Z}_n(\omega)$ tends to $\tau(\omega_r)$ as $n \to \infty$. We show that the relative final size $\tau(\omega_r)$ can increase for $\omega_r > 0$ compared to the baseline $\omega_r = 0$ model. We do so by giving a lower bound for $\tau(\omega_r)$. This lower bound is obtained by considering a model with slightly different social distancing rules: suppose a susceptible individual distances him/herself from its infectious neighbour. Then he/she tries to rewire to a randomly chosen individual $v$ in the population. If $v$ is an individual with original degree $d$, then no connection is made and the existing connection is dropped instead. On the other hand, if $v$ has original degree 0, then a connection is made as in the original model. But, $v$ is not allowed to transmit infection to an individual with original degree $d$. Note that all these modifications make infection less likely, so the final size of this modified model is less than that of the original social distancing model. Furthermore, note that in the baseline model without rewiring ($\omega_r = 0$) the final size of

the original model is equal to the lower bound obtained from the modified model.

Previous work [5, Theorem 6 and Proposition 4] yields that the deterministic final fraction of the population with original degree $d$ that becomes infected in the epidemic is $\rho = 1 - z^d$ where $z \in (0,1)$ is the unique solution to

$$(\beta + \omega_r)z - \omega_r - \beta z^{d-1} = 0 \tag{S.2}$$

(note that by considering only the original degree $d$ individuals, the probability generating function in [5] is given by $f_D(s) = s^d$ and $\mu_D = d$). Let $\theta = \omega_r/(\beta + \omega_r)$ denote the probability that social distancing occurs before transmission for a connection between a susceptible and an infectious individual. The fraction of the original degree $d$ population that rewires to outside the largest connected component (with probability $\theta$), then gets infected (the relative final size of the epidemic is $\rho$), and transmits infection (with probability $1-\theta$) to outside the largest connected component is

$$\phi = \rho p_0 \theta(1-\theta) - (1-\rho), \tag{S.3}$$

where $1-\rho$ is the fraction of the original degree $d$ population that escapes infection. Asymptotically, the probability for an individual of degree 0 to escape infection is $(1 - 1/(np_0))^{\phi n p_d} \to e^{-\phi p_d/p_0}$ as $n \to \infty$, since approximately $n\phi p_d$ individuals rewire and transmit infection to an original degree 0 individual, and for each such rewiring event the individual rewired to is chosen uniformly at random from the $np_0$ original degree 0 individuals. Therefore, the fraction of the population that originally had degree 0 that gets infected is approximated by $p_0(1 - e^{-\phi p_d/p_0})$. Hence, the total fraction of the population that eventually gets infected is at least

$$p_d\rho + p_0(1 - e^{-\phi p_d/p_0}). \tag{S.4}$$

The latter yields an asymptotic lower bound for the final fraction infected in the SI epidemic on the configuration network with rewiring rate $\omega_r$ ($\gamma = 0$, $\omega_d = 0$). We consider the first order approximation of (S.4) in $\omega_r$ to show that the lower bound for the relative final size is exact when $\omega_r = 0$ and increasing for small $\omega_r$, thus the final size of the original model also increases for small $\omega_r$. We approximate $\rho$ by considering (S.2). Denote the left-hand side of (S.2) by $F(z(\omega_r), \omega_r)$, so $F(z(\omega_r), \omega_r) = 0$. Then $\partial F/\partial z \cdot z'(\omega_r) + \partial F/\partial \omega_r = 0$, which yields $z'(\omega_r) = -(z-1)/(\beta + \omega_r - \beta(d-1)z^{d-2})$. Hence $z(\omega_r) = z(0) + z'(0)\omega_r + o(\omega_r) = \omega_r/\beta + o(\omega_r)$, and we can approximate $\rho = 1 - (\omega_r/\beta)^d + o(\omega_r^d)$ for $\omega_r > 0$ small enough. Next, we make the approximation $\phi = p_0\omega_r/\beta + o(\omega_r)$ as $\omega_r \downarrow 0$. The first-order approximation of (S.4) is

$$p_d\,(1 + p_0\omega_r/\beta) + o(\omega_r).$$

Recall that the limiting mean fraction infected in the event of a large outbreak in the model with no rewiring ($\omega_r = 0 = \omega_d$) is $p_d$. Thus, since $p_d\,(1 + p_0\omega_r/\beta) \geq p_d$ for all $p_0, \omega_r > 0$, we find that the final fraction infected in case of a major outbreak is increased for all sufficiently small but strictly positive rewiring rates $\omega_r > 0$ for the modified model. In other words, the asymptotic lower bound for the relative final size given a major outbreak is increasing for small $\omega_r > 0$.

Next, we show that the asymptotic lower bound for the expected relative final size has the same property. For the expected relative final size we have

$$E(\bar{Z}(\omega_r)) = 0 + \tau(\omega_r)P_{\omega_r}(\text{major outbreak}) \geq p_d(1 + \frac{p_0}{\beta}\omega_r)P_{\omega_r}(\text{major outbreak}) + o(\omega_r).$$

In order to show that also $E(\bar{Z}(\omega_r))$ has a lower bound that is increasing in $\omega_r$ for sufficiently small $\omega_r$, it suffices to show that $P_{\omega_r}(\text{major outbreak})$ does not decrease too fast. We show that $1 - P_{\omega_r}(\text{major outbreak}) = P_{\omega_r}(\text{minor outbreak}) \leq p_0 + p_d\omega_r^{d-1} + o(\omega_r^{d-1})$ or equivalently that

$$P_\theta(\text{minor outbreak}) \leq p_0 + p_d\theta^{d-1} + o(\theta^{d-1}). \tag{S.5}$$

Note that there is a minor outbreak if either the index case has degree 0 (with probability $p_0$), or the index case has degree $d$ (with probability $p_d = 1 - p_0$) but the outbreak that takes place in the configuration model where all individuals have degree $d$ is a minor outbreak. Consider the configuration model without the degree 0 individuals. We modify the model by letting the index case have degree $d - 1$ and all other individuals have degree $d$. Consequently, *all* individuals, including the index case, have $d - 1$ susceptible neighbours when newly infected in the beginning of the epidemic. This modified model has a probability of a minor outbreak that is larger than the original model (and is exact in the case $\theta = 0$), i.e. $P_\theta(\text{minor outbreak}) \leq P_\theta(\text{minor outbreak of the modified model})$. Let $\pi(\theta)$ denote the probability of a minor outbreak for the modified model, given that the index case is of degree $d-1$ (with probability $p_d = 1-p_0$). By conditioning on the number of neighbours that avoid infection in the first generation, i.e. the number of neighbours that rewire away before infection, we find the consistency

$$\pi(\theta) = \sum_{j=0}^{d-1} \pi(\theta)^{d-1-j} \binom{d-1}{j} \theta^j (1-\theta)^{d-1-j} = \big(\theta + \pi(\theta)(1-\theta)\big)^{d-1}.$$

Note that $\pi(0) = 0$ since a major outbreak will occur without any rewiring. By the Taylor expansion of $\pi(\theta)$ about $\theta = 0$, we find that $\pi(\theta) = \theta^{d-1} + o(\theta^{d-1})$, proving (S.5). Since $E(\bar{Z}(0)) = p_d$, we find a lower bound for the expected relative final size that is increasing for sufficiently small $\omega_r > 0$, and is exact for the baseline model $\omega_r = 0$ without rewiring.

## Section S1.4 The final size in several configuration networks

First, we illustrate the proof for the asymptotic lower bound of Section S1.3 for a configuration network with a specific two-point degree distribution. We assume that individuals have either degree 0 or degree 5 ($p_0 = 1/2 = p_5$) and small recovery rate $\gamma = 0.02$. We consider the effect of social distancing on the final size of the epidemic by comparing the average final sizes with social distance rates $\omega > 0$ to the baseline model in Fig. S1. This figure shows that, both with and without conditioning on a major outbreak, social distancing can lead to an increase in the average final size. In fact, this effect can even be observed when some portion of social distancing is done by simply dropping connections, i.e. when there is a reduction in overall network contacts (both $\omega_d > 0$ and $\omega_r > 0$; in Fig. S1 the ratio $\omega_r/\omega_d = 9$ is chosen). Note that the probability of a major outbreak decreases with $\omega$ (Fig. S1B).

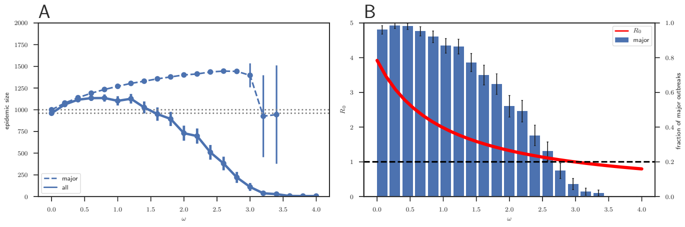


**Figure S1:** Social distancing can lead to an increase in the final size of the epidemic for the configuration network model with degree distribution $p_0 = 1/2 = p_5$. (A) Average final size relative to the average final size in the baseline model (with 95% CI) over all outbreaks and restricted to major outbreaks; dotted horizontal lines are at the size of the epidemic when $\omega = 0$, for reference. (B) $R_0$ as a function of $\omega$ (red curve) and threshold value one (dashed black line) together with the number of outbreaks resulting in a major outbreak (with 95% CI). The average is taken over 250 simulation runs for each parameter value of $\omega$, population size 2000 and one randomly chosen index case with degree 5. The ratio of rewiring over dropping is $\omega_r/\omega_d = 9$, and the recovery rate $\gamma = 0.02$ ($\beta = 1$).

The second type of degree distribution that we consider is again a two-point distribution, but now taking values 1 and 5 ($p_1 = 1/2 = p_5$). Again, we assume $\omega_r/\omega_d = 9$. We let the recovery rate $\gamma = 1.25$ be large (compare with Fig. S1 where the recovery rate is $\gamma = 0.02$), and epidemics are started with 10 randomly chosen infective individuals. The effect of social distancing on the outcome of the epidemic is shown in Fig. S2. One sees that social distancing can increase the average final size compared to the average final size of the baseline model (Fig. S2A). This two-point degree distribution yields a configuration network where there are many components of size 2, i.e. consisting of two individuals that both have degree 1, and one giant component with both individuals of degree 5 and individuals of degree 1 (who have by default exactly one neighbour of degree 5 if part of the giant component). An index case with degree 1 can only cause a major outbreak if he/she is part of the giant component. Note that the large recovery rate implies that the probability that an infectious individual recovers before transmitting to a susceptible neighbour is quite large ($\gamma/(\beta + \gamma) = 0.56$ in the baseline model). If a susceptible individual with degree 5 distances itself from an infectious neighbour, then this individual is likely to still become infected later on in the epidemic due to its high degree. If he/she rewires to a susceptible individual of degree 1, then that degree 1 individual is more likely to become infected as well.

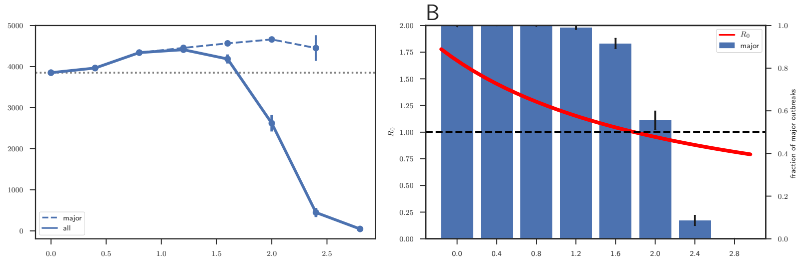


**Figure S2:** The effect of social distancing on the final size of the epidemic for the configuration network model with degree distribution $p_1 = 1/2 = p_5$. (A) Average final size relative to the average final size in the baseline model (with 95% CI) over all outbreaks and restricted to major outbreaks; dotted horizontal lines are at the size of the epidemic when $\omega = 0$, for reference. (B) $R_0$ as a function of $\omega$ (red curve) and threshold value one (dashed black line) together with the number of outbreaks resulting in a major outbreak (with 95% CI). The population size is 5000, and 500 simulation runs are performed for each value of $\omega$. The index case is randomly chosen in the entire population. Recovery rate $\gamma = 1.25$, and ratio of rewiring vs. dropping of $\omega_r/\omega_d = 9$.

Finally, we consider the configuration network model of the main text. We consider the social distancing model on the configuration network with degree distribution $\{p_d\}_{d=0}^{10}$ where $p_d = c/(d + 1)$, $d = 0, 1, \dots, 10$, with $c = 0.331$ the normalization constant. In the main text, each epidemic is initiated with ten initially infected individuals that are randomly chosen from the population. The rational behind this choice is to ensure sufficiently many epidemics result in major outbreaks. Owing to the degree distribution of the population, a large fraction of the population has degree 0 or degree 1. An individual with degree 0 has no connections and is therefore unable to transmit infection in the population. Also an individual with degree 1 is unlikely to generate a major outbreak. In Fig. S3 we compare the final epidemic size for the case that each epidemic starts with 10 randomly chosen infectives to the case that each epidemic starts with only 1 randomly chosen infective.

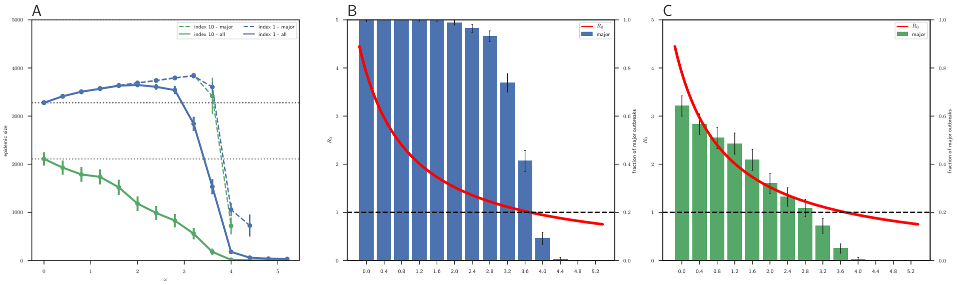


**Figure S3:** The effect of social distancing on the final size of epidemics with different numbers of initially infected individuals. (A) Average final size compared to the average final size in the baseline model (with 95% CI) over all outbreaks (solid line) and restricted to major outbreaks (dashed line); dotted horizontal lines are at the size of the epidemic when $\omega = 0$, for reference. (B) $R_0$ as a function of $\omega$ (red line) and fraction of outbreaks resulting in a major outbreak for the setting of 10 initially infectives (with 95% CI). (C) $R_0$ as a function of $\omega$ (red line) and fraction of outbreaks resulting in a major outbreak for the setting of 1 initially infective (with 95% CI). Black dashed line at $R_0 = 1$ indicates the threshold value for the beginning of the epidemic. We consider the configuration network model with degree distribution $\{p_d\}_{d=0}^{10}$ where $p_d = c/(d+1)$, $d = 0, 1, \ldots, 10$, with $c = 0.331$ the normalization constant. The population size is 5000 and 500 simulation runs are performed for each value of $\omega$. The recovery rate is $\gamma = 0.1$, and $\omega_r/\omega_d = 9$. The index cases are randomly chosen in the entire population. The blue curves show the results for 10 initially infected individuals (results main text Fig. 1) whereas the green curve show the results for one initially infected individual.

Note that the effects of the number of initial infectives as shown in Fig. S3 are not surprising. The average final size over all outbreaks is much smaller in the setting where epidemics are initiated by one initial infective individual. Since this individual is randomly chosen over the entire population, it is quite likely that he/she has degree 0 or 1. In such cases, epidemics will (most likely) die out (Fig. S3C). By considering 10 initial infectives instead, it becomes more likely that an epidemic outbreak occurs (Fig. S3B). This is both because there are simply more infectives to start with, making it less likely that the epidemic dies out owing to stochastic effects, and it being more likely that some initial infectives have higher degree, enabling further transmission in the population. On the other hand, the average final size in case of a major outbreak does not depend on the initial number of infectives (Fig. S3A, blue and green dashed lines).

# Section S2 The clique-network model

In the main text as well as in this supplement we consider the clique-network model where all cliques consist of exactly three individuals. The reason for this choice is that it allows us to illustrate our point that social distancing can have a negative effect on the initial stages of an outbreak by increasing the epidemic threshold parameter $R_*$. At the same time, the choice of cliques of size three simplifies the bookkeeping in the calculations below. Moreover, it yields an explicit expression for the clique reproduction number $R_*$. However, in principle similar calculations can be done also for clique sizes larger than three, or having variable clique sizes.

The clique network with variable clique sizes can be constructed as follows (see also [2, 3] where the same model is referred to as household-network models). A clique-size distribution $\{\pi_h\}$ is predefined that describes the sizes of cliques in the population. The population can be divided into cliques with this distribution by drawing random sizes $h_1, h_2, \ldots$ independently from $\{\pi_h\}$, then labelling all individuals 1 up to $n$, and letting the first $h_1$ individuals make up clique

1, the next $h_2$ individuals make up clique 2, and so on. In the final network, individual 1 is then connected to all individuals he/she is connected to from the construction of the configuration model and individuals 2 up to $h_1$ from the clique construction, and so on.

We denote the degree distribution for the global network connections by $\{p_d\}$, and the mean and variance by $\mu_D$ and $\sigma_D^2$, respectively. We also use the size-biased degree distribution $\{\tilde{p}_d\}$ with $\tilde{p}_d = dp_d/\mu_D$. We let $\tilde{\mu}_D$ denote the mean of the size-biased degree distribution, where $\tilde{\mu}_D = \sum_{d=1}^{\infty} d\tilde{p}_d = \sum_{d=1}^{\infty} d^2 p_d/\mu_D = \mu_D + \sigma_D^2/\mu_D$.

## Section S2.1 Derivation of the epidemic threshold parameter $R_*$

We consider the clique reproduction number $R_*$ that can be interpreted as the expected number of secondary cliques generated by one typical newly infected clique at the beginning of an epidemic [6, 1, 4]. So, rather than considering individuals as the units of interest we consider cliques. The clique reproduction number $R_*$ satisfies the desired threshold behaviour that, as the number of cliques tends to infinity, there is a strictly positive probability of a major outbreak if $R_* > 1$ and only minor outbreaks occur if $R_* \leq 1$.

At the start of an epidemic there are only few infected individuals and most individuals are susceptible. Therefore, a newly infected clique at the beginning of an epidemic has most likely only one newly infected individual that got infected by a neighbour outside his/her own clique. In the SIR epidemic on the clique-network with social distancing, there are exactly two types of newly infected clique: the first infected individual in the clique was infected through (1) a global network neighbour or (2) a rewired network neighbour. Note that in case (1) the individual has $d-1$ susceptible global connections with probability $\tilde{p}_d$ while in case (2) the individual has $d$ susceptible global connections with probability $p_d$ (note that the probability that an individual is rewired to more than once is negligible in the early stages). The other two clique members have $d$ susceptible global connections with probability $p_d$.

The clique reproduction number $R_*$ is given by the dominant eigenvalue of the $2 \times 2$ matrix $K = (K_{ij})_{i,j=1,2}$, where $K_{ij}$ is the expected number of cliques of type $j$ generated by one newly infected clique of type $i$. In the remainder of this section we derive expressions for the $K_{ij}$ by considering all possible events that can occur within the clique. We denote the clique member that was infected from outside of the clique by $u_*$. The other two clique members are denoted by $u_1$ and $u_2$. We let

$$\theta_1 = \frac{\beta}{\beta+\omega+\gamma}, \quad \theta_2 = \frac{\omega}{\beta+\omega+\gamma}, \quad \theta_3 = 1-\theta_1-\theta_2 = \frac{\gamma}{\beta+\omega+\gamma},$$

so that $\theta_1$ is the probability that transmission occurs from an infectious individual to a given susceptible connection before recovery or social distancing, $\theta_2$ is the probability that social distancing occurs before transmission or recovery, and $\theta_3$ is the remaining probability (of recovery before either event).

The $K_{ij}$ can be derived directly from the above interpretation. First of all, note that $K_{12} = K_{22}$, i.e. the expected number of secondary cliques of type 2 generated by a newly infected clique does not depend on the type of that clique as the global network degree of $u_*$ does not play a role. A clique member within a clique can transmit infection to individuals in another clique through a rewired edge if (i) there is at least one clique edge that is rewired away to a new individual in the population, (ii) the individual $u_1$ that rewires away becomes infected by a clique member, and (iii) $u_1$ transmits infection along its rewired clique connection. Since we need both that clique connections rewire to new cliques and the individuals that rewire away to become infected, the only possibility for secondary cliques of type 2 to be generated is if there is exactly one rewired clique connection in the index clique.

When $u_*$ is newly infected and the other two clique members $u_1$ and $u_2$ are (still) susceptible, the following events can occur: (i) $u_*$ recovers (at rate $\gamma$), (ii) $u_*$ transmits to $u_1$ or $u_2$ (at rate $2\beta$), or (iii) $u_1$ or $u_2$ distances itself from $u_*$ (at rate $2\omega$). So we find that the probability that $u_*$ transmits to $u_1$ is

$$\pi = \frac{\beta}{\gamma + 2\beta + 2\omega}. \tag{S.6}$$

The other probabilities in the derivations below can be derived in similar manner and we leave out the details. We find the following two possibilities.

- $u_*$ transmits to $u_1$ with probability $\pi$, then $u_2$ rewires one of its clique connections from either $u_*$ or $u_1$ (with probability $2\omega_r/(2\beta + 2\omega + 2\gamma)$), after which $u_2$ becomes infected through its clique connection that was not rewired away (with probability $\theta_1$). Finally, $u_2$ transmits to a global neighbour through its rewired clique edge (with probability $\theta_1$)

- $u_1$ rewires away from $u_*$ to a new individual (with probability $2\omega_r/(2\beta+\gamma+2\omega)$), then $u_*$ transmits to $u_2$ (with probability $\theta_1$). Next, $u_2$ transmits infection to $u_1$ (with probability $\theta_1$), and $u_1$ transmits to a global neighbour through its rewired clique edge (with probability $\theta_1$)

Therefore,

$$K_{12} = \frac{4\omega_r}{(2\beta + \gamma + 2\omega)}\theta_1^3 = K_{22}. \tag{S.7}$$

$K_{11}$ and $K_{21}$ are a bit more involved as there are more possibilities to take into account. Note that the only difference between the two $K_{i1}$ is in the degree of $u_*$. We note that the expected number of newly infected cliques generated by network edges of $u_*$ is the probability $\theta_1$ of transmission through a network connection (before recovery of $u_*$ or rewiring of network edges) times the expected number of susceptible network neighbours of $u_*$. If $u_*$ is of type 1, then the expected number of susceptible network neighbours is $\tilde{\mu}_D - 1$. If $u_*$ is of type 2, then this expected number is $\mu_D$.

Next, we note that clique members $u_1$ and $u_2$ are interchangeable in the sense that they both have network degree $d$ with probability $p_d$, and all three clique members $u_1$, $u_2$, and $u_*$ are connected to each other. If individual $u_1$ gets infected, then the expected number of susceptible network neighbours it has is $\mu_D$. The expected number of secondary cases an infectious clique member $u_1$ generates is then $\theta_1\mu_D$. We derive the probability that $u_1$ becomes infected by taking into account all relevant events and the order in which they occur.

The following events can occur (with corresponding probabilities):

- $u_*$ transmits to $u_1$ with probability $\pi$

- $u_*$ transmits to $u_2$ with probability $\pi$, after which $u_*$ or $u_2$ transmits to $u_1$ with probability $\frac{2\beta}{2\gamma+2\beta+2\omega} = \theta_1$.

- $u_*$ transmits to $u_2$ with probability $\pi$, then $u_1$ distances itself from either $u_*$ or $u_2$ with probability $\theta_2$, and finally $u_1$ becomes infected by the clique member it did not distance itself from with probability $\theta_1$

- $u_*$ transmits to $u_2$ with probability $\pi$, then $u_*$ or $u_2$ recovers with probability $\theta_3$, and finally $u_1$ becomes infected by the clique member that is still infectious with probability $\theta_1$

- $u_2$ distances itself from $u_*$ with probability $\frac{\omega}{\gamma+2\beta+2\omega}$ after which $u_*$ transmits to $u_1$ with probability $\theta_1$
- $u_1$ distances itself from $u_*$ with probability $\frac{\omega}{\gamma+2\beta+2\omega}$, then $u_*$ transmits to $u_2$ with probability $\theta_1$, and finally $u_2$ transmits to $u_1$ with probability $\theta_1$

The probability that $u_2$ becomes infected is obtained by interchanging the names $u_1$ and $u_2$, so we simply multiply by a factor 2 in the expected number of infected cliques generated by $u_1$ and $u_2$.

Putting these pieces together, we find that the expressions for the $K_{ij}$, $i, j = 1, 2$, are as follows:

$$\begin{aligned} K_{11} &= \theta_1(\tilde{\mu}_D - 1) + 2\theta_1\mu_D \left( \frac{\beta}{\gamma+2\beta+2\omega} + \frac{\beta}{\gamma+2\beta+2\omega}\theta_1 + \frac{\beta}{\gamma+2\beta+2\omega}\theta_1\theta_2 \right. \\ &\qquad \left. + \frac{\beta}{\gamma+2\beta+2\omega}\theta_3\theta_1 + \frac{\omega}{\gamma+2\beta+2\omega}\theta_1 + \frac{\omega}{\gamma+2\beta+2\omega}\theta_1^2 \right) \\ &= \theta_1(\tilde{\mu}_D - 1) + 2\theta_1\mu_D \left( \frac{\beta}{\gamma+2\beta+2\omega}(1+\theta_1+\theta_1\theta_2+\theta_1\theta_3) + \frac{\omega}{\gamma+2\beta+2\omega}\theta_1(1+\theta_1) \right) \\ K_{21} &= \theta_1\mu_D + 2\theta_1\mu_D \left( \frac{\beta}{\gamma+2\beta+2\omega}(1+\theta_1+\theta_1\theta_2+\theta_1\theta_3) + \frac{\omega}{\gamma+2\beta+2\omega}\theta_1(1+\theta_1) \right) \end{aligned}$$

Note that the sum $2\frac{\omega}{(\gamma+2\beta+2\omega)}\theta_1^2 = \frac{\beta}{\gamma+2\beta+2\omega}\theta_1\theta_2 + \frac{\omega}{\gamma+2\beta+2\omega}\theta_1^2$ of the two terms $\frac{\beta}{\gamma+2\beta+2\omega}\theta_1\theta_2$ and $\frac{\omega}{\gamma+2\beta+2\omega}\theta_1^2$ in $K_{11}$ and $K_{21}$ is the probability of social distancing of an initially susceptible clique member that later becomes infected.

Finally, the clique reproduction number $R_*$ is the dominant eigenvalue of the $2\times 2$ matrix $K = (K_{ij})_{i,j=1,2}$. Therefore, we have an explicit expression of $R_*$ in terms of the model parameters:

$$R_* = \frac{\text{tr} + \sqrt{\text{tr}^2 - 4\text{det}}}{2}, \qquad \text{(S.8)}$$

where tr$= K_{11} + K_{22}$ and det$= K_{11}K_{22} - K_{12}K_{21}$ denote the trace and determinant of the matrix $K$, respectively.

## Section S2.2 Social distancing can increase $R_*$ but this depends on the network structure

We consider two degree distributions for the degree $D$ of the global network, and using (S.8) for $R_*$, show that $R_*$ *can* increase for sufficiently small distancing rate $\omega > 0$ and recovery rate $\gamma > 0$. We consider a third choice for $D$ to show that this need not always be the case. Assume that $\gamma = 0 = \omega_d$ and write $R_* = R_*(\omega_r)$.

First, suppose that $p_1 = p = 1 - p_0$. Then $\mu_D = p$ and $\mu_{\tilde{D}-1} = 0$. Then $R_*(0) = 2p$ and $R_*'(0) = (3 - 2p)/\beta$. In particular, if $p = 1/2$, then $R_*(0) = 1$, and $R_*'(0) > 0$. Therefore, for sufficiently small $\gamma, \omega_d > 0$, an increasing rewiring rate $\omega_r > 0$ can push the epidemic threshold parameter $R_*$ from below to above the threshold value of one as shown numerically in Fig. S4A and Fig. 2C of the main text.

Next, suppose that $D$ is Poisson with mean $\mu_D$. Then $\tilde{D} - 1$ is also Poisson with mean $\mu_D$. Then $R_*(0) = 3\mu_D$, and $R_*'(0) = (2 - 3\mu_D)/\beta$. In particular, if $\mu_D = 1/3$, then $R_*(0) = 1$, and $R_*'(0) > 0$. Thus, for sufficiently small $\gamma, \omega_d > 0$ and $\mu_D$ close to 1/3, an increasing rewiring rate $\omega_r > 0$ can push the epidemic threshold parameter $R_*$ from below to above the threshold value of one as shown numerically in Fig. S4A.

Finally, to show that the result for $R_*$ does not hold in general, we consider the following distribution. Suppose that $p_d = 1$, for some fixed $d > 1$, so all individuals have degree $d$. Then $\mu_D = d$ and $\mu_{\tilde{D}-1} = d - 1$, whence $R_*(0) = 3\mu_D - 1$ and $R'_*(0) = -(1 - 12\mu_D + 9\mu_D^2)/(\beta(3\mu_D - 1)$. Note that $1 - 12\mu_D + 9\mu_D^2 = (3\mu_d - 2)^2 > 0$ as $d > 1$. We find that $R'_*(0) < 0$ for $d > 1$. This shows that rewiring decreases the epidemic threshold parameter $R_*$ for sufficiently small $\omega_r > 0$ (and $\omega_d, \gamma > 0$) as illustrated in Fig. S4B.

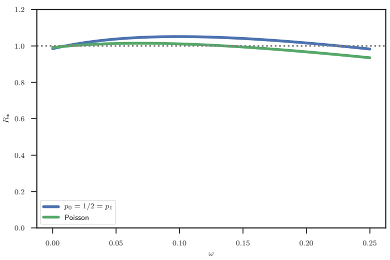


**Figure S4:** $R_*$ for the clique-network model with cliques of size 3 with mean infectious period $1/\gamma = 100$ time units ($\beta = 1$ per time unit), $\omega_r/\omega_d = 9$ (A) Social distancing can increase the epidemic threshold parameter $R_*$ from below to above its threshold value of one for clique-network models. Illustration with two-point degree distribution with $p_0 = 1/2 = p_1$ (blue line) and Poisson degree distribution with mean $\mu_D = 0.335$ (green line) (B) Social distancing does not have to increase the epidemic threshold parameter $R_*$. Illustration with degree distribution $p_3 = 1$.

# Section S3 Real-world networks

## Section S3.1 Properties of the real-world networks

We summarize the most important characteristics of the real-world networks for our purpose, other network summary statistics and more details are found in [9].

The ‘arXiv General Relativity collaboration’ network describes scientific collaborations between authors that submitted papers to the arXiv in the General Relativity and Quantum Cosmology category. Edges between nodes represent two co-authors that have written a paper together. There are 5241 nodes and 14484 edges in the network. In total there are 354 connected components that make up the network and the largest connected component covers a fraction of 0.793 nodes and 0.926 edges. The minimum and maximum degree in the population are 1 and 81, with a mean of 5.53 and a variance of 62.7. The median degree is 3. There are in total 777 nodes with degree 3, and out of these nodes, 676 are part of the largest connected component. We choose the index case at random from these 676 nodes.

In the ‘Facebook social circles’ network, nodes are survey participants of the social network website Facebook that were using a specific app. Edges between nodes represent the ‘circles’ or ‘friends lists’ of those participants. There are 4039 nodes and 88234 edges. The largest network component is precisely the network itself. The minimum and maximum degree in the population are 1 and 1045, with a mean of 43.70 and a variance of 2748.44. The median degree in the population is 25, and there are 55 individuals with this median degree of 25. We choose an index case at random from this set of individuals.

## Section S3.2 Social distancing on the collaboration network with long mean infectious period

In the main text, we demonstrate that social distancing increases the final size of the epidemic when considering relatively short mean infectious periods (large recovery rate $\gamma$); see Fog. 3. The same statement for the final size of the epidemic holds for much longer mean infectious periods, see Fig. S5. Shorter mean infectious periods make it less likely for an infectious individual to transmit to his/her contacts, making major outbreaks less likely to occur. In this way, the average final size is smaller than in the setting with longer mean infectious periods (given the same transmission rate); compare Fig 3 to Fig. S5.

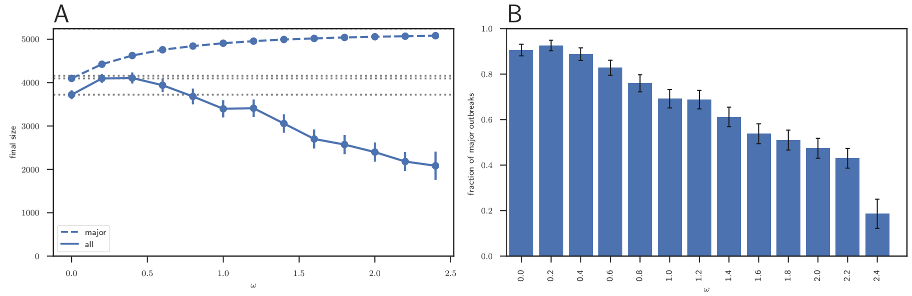


**Figure S5:** Social distancing can increase the final size of the epidemic on real-world networks for small recovery rates. (A) The average final size with and without conditioning on a major outbreak (with 95% CI); dotted horizontal lines are for comparison with the size at $\omega = 0$.(B) Fraction of all outbreaks that resulted in major outbreaks (with 95% CI). Simulated SIR epidemic with recovery rate $\gamma = 0.05$ ($\beta = 1$) and social distancing $\omega_r/\omega_d = 9$ over 500 simulation runs for each value of $\omega$ on the collaboration network of arXiv General Relativity with randomly chosen index case with median degree that is part of the largest connected component of the network.

# Section S4 Simulation studies of the social distancing model

We are interested the epidemic final size and the probability of a major outbreak for the social distancing model applied to (i) the configuration network model, (ii) the clique network model, and (iii) two real-world networks. The social distancing model is mathematically challenging to analyse. Although we have some analytical results (presented in Sections Section S1 and Section S2), e.g. for the threshold parameter $R_0$ for the configuration network model and $R_*$ for the clique network model, other quantities of interest, i.e. the final size and the probability of a major outbreak we have not managed to characterize mathematically. Moreover, on large real-world networks it is impractical to exactly compute the quantities we are interested in. The results in this text are obtained through simulation methods.

Given the structure of the networks it is fairly straightforward (since the epidemic process is a continuous-time Markov chain) to write code to simulate realisations of the final size of stochastic SIR epidemic process described in section *Model description* of the main article. By inspecting histograms of these simulated final sizes we find that the cut-off of 10% of population size (as stated in section *Model description* of the main text) is satisfactory for the networks we consider.

In plots depicting the results of simulations we present point estimates, for example the

proportion of simulations that result in a final size greater than 10% of population size as an estimate of major outbreak probability, the mean final size amongst outbreaks with a final size greater than 10% of population size as an estimate of the relative final size of a major outbreak. We also present confidence intervals (CI) around these estimates in cases where those intervals are large enough to be visible on the scales used in the plots.

# References


[1] F. Ball, D. Mollison, and G. Scalia-Tomba. Epidemics with two levels of mixing. *Ann. Appl. Probab.*, 7(1):46–89, 1997.

[2] F. Ball, D. Sirl, and P. Trapman. Threshold behaviour and final outcome of an epidemic on a random network with household structure. *Adv Appl Probab*, 41:765–796, 2009.

[3] F. Ball, D. Sirl, and P. Trapman. Analysis of a stochastic SIR epidemic on a random network incorporating household structure. *Math Biosci*, 224:53–73, 2010.

[4] F. Ball, L. Pellis, and P. Trapman. Reproduction numbers for epidemic models with households and other social structures II: Comparisons and implications for vaccination. *Math. Biosci.*, 274:108–139, 2016.

[5] F. Ball, T. Britton, K. Y. Leung, and D. Sirl. An SIR network epidemic model with preventive dropping of edges. *in preparation*, 2018.

[6] N. G. Becker and K. Dietz. The effect of household distribution on transmission and control of highly infectious diseases. *Math. Biosci.*, 127:207–219, 1995.

[7] B. Bollobás. *Random Graphs.* Academic Press, New York, 2001.

[8] T. Britton, D. Juher, and J. Saldaña. A network epidemic model with preventive rewiring: comparative analysis of the initial phase. *Bull Math Biol*, 78:2427–2454, 2016.

[9] Jure Leskovec and Andrej Krevl. SNAP Datasets: Stanford large network dataset collection. `http://snap.stanford.edu/data`, June 2014.
